# Supplementary material for: On the Validity of Modeling SGD with Stochastic Differential Equations (SDEs)
Source: arXiv:2102.12470 source file (2021-06-16)
Supplement: Supplementary file 1 [file addl_appendix.tex]

\section{SDE Approximation implies Linear Scaling Invariance, but the Inverse is False}\label{sec:sde_to_lsi}
We demonstrate this claim through an example. 
\begin{example}
Let $\N^+$ be the domain and each data is sampled from $\mu_\lambda$, where $\mu_\lambda$ is poisson distribution with parameter $\lambda$, $\mu_\lambda(a) = \frac{\lambda^a e^{-\lambda}}{a!}$, $\forall a\in \N$. Let $x\in\R$ and the loss function is simply linear loss, i.e., $\Loss_a(x) = ax$. For batch $\vB = \{a_i\}_{i=1}^m$, we define $\Loss_\vB(x) = \frac{\sum_{i=1}^m a_i}{m}x$. Note that the convolution of two poisson distributions with parameter $\lambda_1,\lambda_2$ is still a Poisson distribution, with parameter $\lambda_1+\lambda_2$. Thus we conclude that starting from $x_0= 0$, with learning rate $\eta=1$, batch size $B$ and total number of samples $N$ (we assume $B$ divides $N$), we have 
\[ \forall 1\le k\le \frac{N}{B},\ \ x_k = x_{k-1} - \eta \nabla\Loss_{\vB_k}(x_{k-1})\quad \Longrightarrow\quad -\frac{\eta}{B}x_{\frac{N}{B}} \sim\mu_{N\lambda}. \quad\quad\quad\]

Therefore, LSR holds exactly --- as long as the $\frac{\eta}{B}$ is fixed, the resulting distribution of $x_{\frac{N}{B}}$ is independent of individual value of $B$ or $\eta$ and it's clear that the distribution is Poission but not Gaussian, thus is not close to the SDE,~\Cref{eq:motivating_sde}.  Also this is an example where moving towards each side of LSR doesn't make the dynamics closer to the SDE,~\Cref{eq:motivating_sde}. \footnote{Here we used the Possion process and indeed any Levy process would work.}
\end{example}

 The above example shows that tiny learning rate plus  matched the first and second moments is not sufficient for SGD,~\Cref{eq:sga_iter}, to be close to SDE,~\Cref{eq:motivating_sde}. As we will see from the proof later(e.g.\Cref{lem:D}), it also requires the third order moment to vanish.
